# Supplementary material for: HOIGPT: Learning Long Sequence Hand-Object Interaction with Language Models
Source: arXiv:2503.19157 source file (2025-03-24)
Supplement: Supplementary file 1 [file X_suppl.tex]

\clearpage
\setcounter{page}{1}
\maketitlesupplementary
\appendix
% \begin{abstract}
% In this supplementary material, we included additional qualitative results for ablation studies and comparison with other method.
% \end{abstract}

\section{Details of HOI-decomposed VQ}
In this section, we provide details of our proposed HOI-decomposed VQ. Using the inputs from the hand and object encoders, the HOI-decomposed VQ gradually learns the residual $\z_{res}$ from the learned subject and finally outputs the predicted HOI latent feature $\hat{z}$.
\begin{algorithm}[h]
\DontPrintSemicolon
\caption{HOI-decomposed VQ}\label{algo:rvq}
\SetKwInput{Input}{Input}
\SetKwInput{Output}{Output}
\Input{$z_o, z_l, z_r$: the output of the encoders, vector quantizers $Q_i$ for $i \in \{o,l,r\}$, object/hand codebooks $C_o$, $C_h$}
\Output{The quantized HOI feature $\hat{z_N}$} 

$z \gets z_o + z_l + z_r$\; 
$\hat{z} \gets 0.0$\;
${z_{res}} \gets z$\; 

\For{$i$}{
    \If{$i$ is $\{o\}$}{
        $q_i \gets Q_i({\rm C_o}, {z}_{res})$\;
    }
    \Else{
        $q_i \gets Q_i({\rm C_h}, {z}_{res})$\;
    }
    ${z} \mathrel{+}= q_i$\;
    ${z}_{res} \mathrel{-}= q_i$\;
}
\Return $\hat{z}$
\end{algorithm}

% \begin{algorithm}[ht]
% \caption{Residual Vector Quantization}
% \label{alg:rvq}
% \begin{algorithmic}[1]
% \Require $y = \text{enc}(x)$ \Comment{the output of the encoder}
% \Require vector quantizers $Q_i$ for $i = 1..N_q$
% \Ensure the quantized $\hat{y}$
% \State $\hat{y} \gets 0.0$
% \State $\text{residual} \gets y$
% \For{$i = 1$ to $N_q$}
%     \State $\hat{y} \mathrel{+}= Q_i(\text{residual})$
%     \State $\text{residual} \mathrel{-}= Q_i(\text{residual})$
% \EndFor
% \State \Return $\hat{y}$
% \end{algorithmic}
% \end{algorithm}

\section{Additional Qualitative Results}
In this supplementary material, we present additional qualitative results for ablation studies and comparison with other methods, including Text2HOI~\cite{guo2022tm2t}, MotionGPT~\cite{jiang2024motiongpt} and T2MGPT~\cite{zhang2023generating}. Please refer to the attached video for these qualitative results.

\section{Implementation Details}
We included additional details about the hyper-parameters and evaluation.

\myheading{Hyper-parameters}. We set the $\lambda = 0.2, \beta = 0.5, \gamma = 1$ and $\alpha = 0.5$ in our experiments. \\
\myheading{Evaluation metric}. We follow \cite{guo2022generating} to train the HOI text matching network for feature extraction. Similarly, the motion encoder and text encoder are two bidirectional GRUs. We train the feature extractor for 65 epochs in our combined dataset for evaluation.

\section{Dataset Details}
We provide additional details about the dataset we used to train and evaluate HOIGPT. Our combined dataset includes two popular HOI datasets: GRAB~\cite{taheri2020grab} and Arctic~\cite{fan2023arctic}, comprising a total of 6.1k HOI sequences with 65 unique objects (\textit{Box, Capsule Machine, Espresso Machine, Ketchup, Laptop, Microwave, Mixer, Notebook, Phone, Scissors, Waffle Iron, Airplane, Alarm Clock, Apple, Banana, Binoculars, Body, Bowl, Camera, Coffee Mug, Cube Large, Cube Medium, Cube Small, Cup, Cylinder Large, Cylinder Medium, Cylinder Small, Doorknob, Duck, Elephant, Eyeglasses, Flashlight, Flute, Frying Pan, Game Controller, Hammer, Hand, Headphones, Knife, Lightbulb, Mouse, Mug, Phone, Piggy Bank, Pyramid Large, Pyramid Medium, Pyramid Small, Rubber Duck, Scissors, Sphere Large, Sphere Medium, Sphere Small, Stamp, Stanford Bunny, Stapler, Table, Teapot, Toothbrush, Toothpaste, Torus Large, Torus Medium, Torus Small, Train, Watch, Water Bottle, Wine Glass, Wristwatch}). From this dataset, 500 samples, including unseen HOI sequences and objects, were selected for testing.
